# Supplementary material for: (Bandit) Convex Optimization with Biased Noisy Gradient Oracles
Source: arXiv:1609.07087 source file (2020-07-04)
Supplement: Supplementary file 1 [file appendix.tex]

%!TEX root =  bgo_cam_ready.tex
% please do not delete or change the first line (needed by Csaba's editor)

\section{Reduction of Oracles}
\label{sec:orrel}
\input{red_proof}

\section{Gradient Estimation}
\label{sec:appendix-grad}
\input{appendix-grad.tex}

\section{Upper Bound Proof}
\label{sec:appendix-md}
\input{appendix-upperbds.tex}

\section{Lower Bound Proof}
\label{sec:appendix-lb-proof}
\input{lb_proof}
